# Supplementary material for: Robustness Assessment of Complex Networks using the Idle Network
Source: arXiv:2206.00062 source file (2022-05-31)
Supplement: Supplementary file 1 [file Engsig_etal22_SM.pdf]

# Supplemental Material:
# Robustness Assessment of Complex Networks using the Idle Network

Marcus Engsig
*Department of Science and Engineering, Sorbonne University Abu Dhabi, Abu Dhabi, United Arab Emirates.*

Alejandro Tejedor
*Department of Science and Engineering, Sorbonne University Abu Dhabi, Abu Dhabi, United Arab Emirates. and Department of Civil and Environmental Engineering, University of California, Irvine, Irvine, CA 92697, USA*

Yamir Moreno
*Institute for Biocomputation and Physics of Complex Systems (BIFI), Universidad de Zaragoza, 50018 Zaragoza, Spain*
*Departamento de Física Teórica, Universidad de Zaragoza, 50009 Zaragoza, Spain and*
*Institute for Scientific Interchange, ISI Foundation, Turin, Italy*

This supplemental material provides the extended results of all the experiments performed during this work, demonstrating the validity of our central hypothesis tested, namely, the Idle network contains pertinent and non-redundant information about network robustness, improving its assessment accuracy. Moreover, the results systematically support that including both Active and Idle indicators in a model to estimate network robustness allows the model to better assimilate the variability in the training set, reducing the decline in network robustness assessment as that variability increases. Finally, our experiments using real-world network topologies shed light on the potential of models informed both by active and idle indicators estimating network robustness even for foreign attacks to those included in the training set.

This document is structures as follows:

- In *Section A*, we show the estimation accuracy obtained by Artificial Neural Networks with three different types of inputs: (i) only Active indicators, (ii) only Idle indicators, and (iii) both Active and Idle indicators. This triad of models is trained for each of the topologies (Scale-free, Small-World, and Random), attacks (targeted degree, random spreading, and random), and link densities (initial average degree: $\bar{k} = 3, 6, 12,$ and $24$). We denote these neural networks as *specifically trained neural networks* since each model is trained using a set consisting of a single specific topology, attack, and link density.
- In *section B*, we present results showing the accuracy of the triad of Neural Networks (only using Active indicators, only using Idle indicators, and using both Active and Idle indicators) when the training data set includes a larger variability introduced by generalizing the attack strategies (targeted degree, random spreading and random) and the network topology (Scale-free, Small-World, and Random) for a specific link density.
- *Section C* shows the extended results of our study by fully generalizing the training set, which includes all the topologies, attacks, and densities considered in this study. The estimation accuracy of network robustness by neural network using the generalized training set is evaluated systematically for the different cases and depending on whether only active, idle or both types of indicators were used as input to the Neural Networks.
- In *section D*, we compare the performance of the different neural networks trained with data sets of increased variability (specifically trained, trained under generalized topology and attacks, and trained with the fully generalized dataset). This comparative is used to interrogate the effect of variability of training set in the deterioration of estimation accuracy of robustness.
- In *section E*, we finally present the complementary results of those shown in Fig. 4 in the main manuscript, providing the network robustness estimation accuracy for other three real-world network topologies (Budapest Connectome, Top 500 US airports, and a power grid). These estimations were obtained with Neural Networks using training and validation sets consisting of stochastic degree attacks for two different testing sets: stochastic degree attacks and stochastic betweenness attacks, to show the ability of the different Neural Networks to provide estimations of robustness for previously seen (degree) and unseen (betweenness) attacks.

Note that all the neural networks used are forward-feeding and back-propagating artificial neural networks with three hidden layers of ten neurons per layer, each with ReLu activation functions; set to optimize validation squared residual

loss. Each neural network used in the different sections was implemented with a dataset of 200 attack sequences, with a 3/4 train, 1/8 test, and 1/8 validation split. The neural network's output is the estimation of the efficiency as the proxy for robustness.

## Section A: Specifically Trained Neural Networks

This section presents the network robustness accuracy for *specifically* trained neural networks, which are trained with a dataset of stochastically generated specific topologies, undergoing a single attack strategy for a particular link density. Table S1 displays the sum of squared residuals (*SSR*) for all specific neural networks applied to all 36 combinations of topology, attack, and link density.

Table S1 results demonstrate that Neural Networks informed by both Active and Idle indicators outperform the predictions of Neural Networks fed by only Active or Idle indicators in every single case. This systematically proves our hypothesis. Moreover, we notice that the gain from including the Idle indicators ranges drastically. The lowest gain of 20% comes from the scale-free topology undergoing degree attack with a $\bar{k} = 24$, and the most significant gain of around 900% comes from the scale-free topology undergoing random attack with a $\bar{k} = 3$. The difference in information gained from including the Idle indicators increases as the variability in the dataset grows. The scale-free topology undergoing random attack has the most internal variability in the evolution of the efficiency, as the importance of each node scales as a power law. Therefore, when a series of random attacks are performed, the evolution of the efficiency is significantly different depending on when central hubs are removed during the attack sequence.

| | | **Scale-Free** | | | **Small-World** | | | **Random** | | |
|---|---|---|---|---|---|---|---|---|---|---|
| | | **Degree** | **Spreading** | **Random** | **Degree** | **Spreading** | **Random** | **Degree** | **Spreading** | **Random** |
| $\bar{k} = 3$ | **Active** | 0.02 ± 0.03 | 0.20 ± 0.13 | 3.79 ± 3.47 | 0.01 ± 0.01 | 0.13 ± 0.12 | 0.04 ± 0.03 | 0.01 ± 0.02 | 0.09 ± 0.10 | 0.06 ± 0.03 |
| | **Idle** | 0.10 ± 0.10 | 0.47 ± 0.29 | 6.15 ± 5.16 | 0.03 ± 0.05 | 0.25 ± 0.23 | 0.14 ± 0.08 | 0.05 ± 0.07 | 0.17 ± 0.15 | 0.15 ± 0.10 |
| | **Active + Idle** | 0.01 ± 0.01 | 0.10 ± 0.09 | 0.42 ± 0.29 | 0.01 ± 0.03 | 0.08 ± 0.06 | 0.03 ± 0.02 | 0.006 ± 0.004 | 0.05 ± 0.10 | 0.03 ± 0.02 |
| $\bar{k} = 6$ | **Active** | 0.04 ± 0.05 | 0.12 ± 0.07 | 0.67 ± 0.50 | 0.02 ± 0.01 | 0.06 ± 0.04 | 0.04 ± 0.02 | 0.02 ± 0.01 | 0.05 ± 0.03 | 0.04 ± 0.03 |
| | **Idle** | 0.11 ± 0.011 | 0.33 ± 0.21 | 0.42 ± 0.33 | 0.04 ± 0.02 | 0.14 ± 0.11 | 0.09 ± 0.06 | 0.06 ± 0.04 | 0.12 ± 0.09 | 0.12 ± 0.10 |
| | **Active + Idle** | 0.03 ± 0.02 | 0.07 ± 0.05 | 0.27 ± 0.21 | 0.01 ± 0.004 | 0.02 ± 0.01 | 0.02 ± 0.006 | 0.003 ± 0.002 | 0.01 ± 0.01 | 0.01 ± 0.004 |
| $\bar{k} = 12$ | **Active** | 0.02 ± 0.01 | 0.08 ± 0.04 | 0.92 ± 0.57 | 0.02 ± 0.02 | 0.06 ± 0.05 | 0.04 ± 0.02 | 0.01 ± 0.01 | 0.05 ± 0.04 | 0.06 ± 0.07 |
| | **Idle** | 0.06 ± 0.05 | 0.13 ± 0.08 | 0.45 ± 0.26 | 0.06 ± 0.05 | 0.14 ± 0.10 | 0.13 ± 0.08 | 0.05 ± 0.03 | 0.12 ± 0.09 | 0.13 ± 0.13 |
| | **Active + Idle** | 0.01 ± 0.006 | 0.05 ± 0.03 | 0.17 ± 0.14 | 0.01 ± 0.006 | 0.02 ± 0.01 | 0.01 ± 0.009 | 0.002 ± 0.001 | 0.02 ± 0.02 | 0.03 ± 0.02 |
| $\bar{k} = 24$ | **Active** | 0.01 ± 0.01 | 0.05 ± 0.02 | 0.70 ± 0.75 | 0.04 ± 0.03 | 0.09 ± 0.07 | 0.09 ± 0.09 | 0.02 ± 0.02 | 0.10 ± 0.15 | 0.06 ± 0.08 |
| | **Idle** | 0.04 ± 0.01 | 0.1 ± 0.09 | 0.19 ± 0.12 | 0.07 ± 0.05 | 0.16 ± 0.14 | 0.15 ± 0.12 | 0.07 ± 0.05 | 0.17 ± 0.18 | 0.15 ± 0.14 |
| | **Active + Idle** | 0.008 ± 0.008 | 0.04 ± 0.02 | 0.12 ± 0.13 | 0.02 ± 0.02 | 0.03 ± 0.02 | 0.03 ± 0.05 | 0.01 ± 0.005 | 0.05 ± 0.09 | 0.03 ± 0.03 |

**Table S1 -** Sum of squared residuals (SSR) of the estimation of network robustness for the specifically trained neural networks. The results are shown for all the possible combinations of topology, attack schemes, and link densities.

## Section B: Neural Network trained with generalized attack strategies and topologies for a fixed link density.

For completeness, we include the performance of neural networks trained with augmented datasets consisting of a mix of all the attack strategies (degree, spreading, and random) applied to all the topologies (Scale-Free, Small-World, and Random) with a common link density. The performance of those models is interrogated depending on the type of indicators used (only Active, only Idle, or both Active and Idle) when applied to estimate network robustness for each of the 36 combinations of attack, topology, and link density. The results shown in table S2 not only further support our hypothesis but also show, when these values are compared with those shown in table S1, that the deterioration of the accuracy in the estimation of efficiency as function of the variability introduced in the training set is reduced by including both Active and Idle indicators (for more details see section D).

| | | **Scale-Free** | | | **Small-World** | | | **Random** | | |
|---|---|---|---|---|---|---|---|---|---|---|
| | | **Degree** | **Spreading** | **Random** | **Degree** | **Spreading** | **Random** | **Degree** | **Spreading** | **Random** |
| $\bar{k} = 3$ | **Active** | 2.39 ± 0.99 | 1.97 ± 1.64 | 1.48 ± 1.29 | 0.57 ± 0.17 | 0.77 ± 0.34 | 0.57 ± 0.36 | 0.59 ± 0.21 | 0.39 ± 0.29 | 0.30 ± 0.10 |
| | **Idle** | 1.09 ± 0.56 | 0.93 ± 1.69 | 3.69 ± 3.73 | 3.26 ± 1.02 | 1.47 ± 0.51 | 0.58 ± 0.34 | 0.50 ± 0.26 | 2.21 ± 1.18 | 0.46 ± 0.27 |
| | **Active + Idle** | 0.13 ± 0.04 | 0.49 ± 1.07 | 0.60 ± 0.50 | 0.12 ± 0.05 | 0.43 ± 0.80 | 0.24 ± 0.10 | 0.14 ± 0.05 | 0.15 ± 0.12 | 0.11 ± 0.03 |
| $\bar{k} = 6$ | **Active** | 2.08 ± 1.49 | 1.24 ± 0.69 | 1.75 ± 1.59 | 0.40 ± 0.13 | 0.40 ± 0.21 | 0.12 ± 0.05 | 0.44 ± 0.17 | 0.18 ± 0.12 | 0.16 ± 0.09 |
| | **Idle** | 0.38 ± 0.14 | 0.35 ± 0.22 | 1.21 ± 1.13 | 0.50 ± 0.16 | 0.66 ± 0.35 | 0.22 ± 0.10 | 0.14 ± 0.08 | 0.36 ± 0.21 | 0.21 ± 0.19 |
| | **Active + Idle** | 0.03 ± 0.02 | 0.08 ± 0.05 | 0.28 ± 0.17 | 0.02 ± 0.01 | 0.03 ± 0.02 | 0.03 ± 0.02 | 0.01 ± 0.01 | 0.03 ± 0.02 | 0.02 ± 0.01 |
| $\bar{k} = 12$ | **Active** | 1.80 ± 1.57 | 1.30 ± 0.53 | 1.30 ± 1.23 | 0.32 ± 0.09 | 0.23 ± 0.13 | 0.13 ± 0.09 | 0.52 ± 0.17 | 0.16 ± 0.10 | 0.19 ± 0.12 |
| | **Idle** | 0.10 ± 0.05 | 0.18 ± 0.13 | 0.54 ± 0.37 | 0.25 ± 0.16 | 0.27 ± 0.20 | 0.22 ± 0.15 | 0.12 ± 0.05 | 0.24 ± 0.22 | 0.17 ± 0.12 |
| | **Active + Idle** | 0.02 ± 0.01 | 0.06 ± 0.04 | 0.26 ± 0.24 | 0.04 ± 0.02 | 0.02 ± 0.01 | 0.03 ± 0.01 | 0.020 ± 0.003 | 0.02 ± 0.01 | 0.03 ± 0.02 |
| $\bar{k} = 24$ | **Active** | 2.42 ± 2.16 | 1.05 ± 0.40 | 3.46 ± 2.83 | 0.17 ± 0.04 | 0.20 ± 0.17 | 0.15 ± 0.12 | 0.29 ± 0.19 | 0.15 ± 0.14 | 0.12 ± 0.09 |
| | **Idle** | 0.05 ± 0.01 | 0.15 ± 0.12 | 0.81 ± 0.50 | 0.17 ± 0.11 | 0.18 ± 0.17 | 0.21 ± 0.18 | 0.09 ± 0.06 | 0.19 ± 0.17 | 0.22 ± 0.19 |
| | **Active + Idle** | 0.01 ± 0.01 | 0.05 ± 0.03 | 0.63 ± 0.34 | 0.06 ± 0.02 | 0.04 ± 0.02 | 0.05 ± 0.08 | 0.03 ± 0.01 | 0.06 ± 0.07 | 0.06 ± 0.04 |

**Table S2 -** Sum of squared residuals (SSR) of the estimation of network robustness for neural networks trained with a dataset including all the attack strategies and topologies, while maintaining a uniform link density within each training set. The results are shown for all the possible combinations of topologies, attack schemes, and link densities.

## Section C: Fully generalized Neural Networks.

Table S3 shows the performance of the neural networks trained with the augmented dataset consisting of all the attack strategies (degree, spreading, and random) applied to all the topologies (Scale-Free, Small-World, and Random) with all the different link densities ($\bar{k} = 3, 6, 12, 24$). The performance of those models is interrogated depending on the type of indicators used (only Active, only Idle, or both Active and Idle) when applied to estimate network robustness for each of the 36 combinations of attack, topology, and link density.

The values of the sum of the square residuals (*SSR*) obtained from the efficiency (proxy of robustness) estimation done by the models trained with different sets of indicators shown in table S3 highlight the remarkable capacity of the model trained with both Active and Idle indicators in estimating robustness, particularly when compared with the performance of the model granted only with Active information. The outcome of this experiment confirms once more our hypothesis, demonstrating that together the Active and Idle indicators are able to leverage the variability existing in the training set to disentangle the mixing of different topologies, link densities, and attacks existing in the training set to produce fairly accurate estimations for individual combinations. Two further important remarks can be pointed out from table S3: (i) the estimation accuracy of network efficiency (a property of the Active network) done with the model granted only Idle information is comparable to or better than the accuracy offered by the model trained with only Active indicators in more than 60% of the combinations, showing the particular role of Idle information in informing the estimation in the face of enhanced variability; (ii) In particular cases this effect leads to a performance of the Neural Network trained by Active and Idle indicators of the fully generalized compatible or better than the performance offered by the model specifically trained (e.g., see Table S1 for Scale-Free $\bar{k} = 3$ )

The results in table S3, when compared with those shown in tables S1 and S2, show that the deterioration of the accuracy in the estimation of efficiency as a function of the variability introduced in the training set is reduced by including both Active and Idle indicators (for more details see section D).

| | | Scale-Free | | | Small-World | | | Random | | |
|---|---|---|---|---|---|---|---|---|---|---|
| | | **Degree** | **Spreading** | **Random** | **Degree** | **Spreading** | **Random** | **Degree** | **Spreading** | **Random** |
| $\bar{k} = 3$ | **Active** | 7.36 ± 1.70 | 8.45 ± 1.18 | 2.70 ± 2.86 | 4.49 ± 0.55 | 0.72 ± 0.34 | 1.26 ± 0.58 | 5.70 ± 1.30 | 0.84 ± 0.37 | 0.84 ± 0.20 |
| | **Idle** | 1.07 ± 0.59 | 0.50 ± 0.24 | 13.56 ± 6.29 | 4.75 ± 1.42 | 3.21 ± 0.99 | 16.59 ± 1.95 | 5.24 ± 2.21 | 2.62 ± 0.89 | 15.45 ± 2.66 |
| | **Active + Idle** | 0.08 ± 0.04 | 0.24 ± 0.26 | 0.50 ± 0.32 | 0.11 ± 0.03 | 0.40 ± 0.26 | 0.41 ± 0.17 | 0.09 ± 0.02 | 0.17 ± 0.12 | 0.15 ± 0.05 |
| $\bar{k} = 6$ | **Active** | 6.48 ± 2.87 | 6.15 ± 1.91 | 4.00 ± 3.80 | 2.99 ± 0.74 | 1.26 ± 0.53 | 0.66 ± 0.16 | 3.80 ± 0.80 | 0.62 ± 0.26 | 0.64 ± 0.22 |
| | **Idle** | 0.70 ± 0.26 | 0.76 ± 0.40 | 3.03 ± 1.77 | 2.74 ± 0.71 | 0.89 ± 0.34 | 2.77 ± 0.65 | 0.46 ± 0.38 | 0.68 ± 0.30 | 2.88 ± 1.02 |
| | **Active + Idle** | 0.28 ± 0.15 | 0.25 ± 0.10 | 0.73 ± 0.60 | 0.29 ± 0.10 | 0.13 ± 0.05 | 0.67 ± 0.27 | 0.19 ± 0.08 | 0.10 ± 0.04 | 0.24 ± 0.10 |
| $\bar{k} = 12$ | **Active** | 3.81 ± 1.95 | 3.79 ± 1.47 | 4.09 ± 3.04 | 1.76 ± 0.36 | 1.33 ± 0.61 | 0.38 ± 0.13 | 2.83 ± 0.70 | 0.34 ± 0.12 | 0.33 ± 0.08 |
| | **Idle** | 0.27 ± 0.09 | 0.97 ± 0.59 | 1.32 ± 1.14 | 0.32 ± 0.15 | 1.71 ± 0.33 | 0.80 ± 0.24 | 1.70 ± 0.61 | 1.17 ± 0.27 | 0.79 ± 0.22 |
| | **Active + Idle** | 0.19 ± 0.08 | 0.23 ± 0.09 | 0.57 ± 0.31 | 0.19 ± 0.08 | 0.10 ± 0.04 | 0.26 ± 0.09 | 0.20 ± 0.05 | 0.07 ± 0.03 | 0.22 ± 0.08 |
| $\bar{k} = 24$ | **Active** | 2.98 ± 1.37 | 4.65 ± 0.83 | 11.14 ± 5.39 | 1.66 ± 0.23 | 1.28 ± 0.51 | 0.78 ± 0.16 | 2.75 ± 0.26 | 0.91 ± 0.30 | 0.95 ± 0.34 |
| | **Idle** | 0.11 ± 0.04 | 4.70 ± 1.60 | 8.06 ± 3.08 | 1.62 ± 0.29 | 4.08 ± 0.74 | 3.20 ± 0.46 | 3.39 ± 0.69 | 3.9 ± 0.73 | 3.24 ± 0.62 |
| | **Active + Idle** | 0.13 ± 0.03 | 0.56 ± 0.13 | 1.53 ± 0.82 | 0.12 ± 0.06 | 0.09 ± 0.04 | 0.07 ± 0.05 | 0.10 ± 0.03 | 0.10 ± 0.08 | 0.08 ± 0.05 |

**Table S3 -** Sum of squared residuals (SSR) of the estimation of network robustness for neural networks trained with a dataset including all the attack strategies, topologies, and link densities. The results are shown for all the possible combinations of topology, attack scheme, and link density.

## Section D: Deterioration of Estimation Accuracy through Generalization

This section presents a comparative study to estimate the degree of deterioration of the estimation accuracy of network robustness as the variability of the training set is increased by mixing topologies, attacks, and link densities. We evaluate the deterioration of the estimation depending on whether only Active or Idle indicators are included as input to the Neural Network, or if both Active and Idle indicators are provided.

The first obvious and expected observation from the results displayed in Table S4 is that as the variability in the training set is increased, the Neural Network performance declines, as shown by the increasing value of the sum of the square residuals (*SSR*). However, this decline is not comparable for the different Neural Networks trained with the different indicators. The results shown in table S4 clearly indicate that neural networks trained with only Active indicators have a faster rate of deterioration in their estimation of network robustness as the variability in the training set increases. Interestingly, when the neural network is only trained with Idle indicators, its performance, although starting from a lower stand (higher *SSR*), declines at a much lower rate, achieving in many (17/36) instances a higher performance than the Neural Network trained with only Active indicators for the fully generalized training set. More importantly, when both Active and Idle indicators are included in the training set, the neural network's performance is better than the performance of the NN trained with active indicators alone, and its rate of decline in performance is much smaller than in the Active case. Particularly, the case where the estimation accuracy of the Active neural network deteriorates the least is the small world of $\bar{k} = 24$ undergoing a random attack, where it only deteriorates by 0.69. Here, the Active and Idle deteriorates by a mere 0.04. On the other hand, the random topology undergoing degree attack for $\bar{k} = 3$, we observe a deterioration of predictive power of 5.69, where the Active and Idle estimation accuracy only falls by 0.084. Finally, we underline an interesting case, the random topology undergoing random attack with $\bar{k} = 24$, where the estimation done by the neural network trained with the fully generalized training set, both the active and idle fail independently, providing very high values of SSR, but jointly, they provide an exceedingly good estimation, similar to the one obtained from the specifically trained neural network.

To further illustrate our results from table S4, Figs. S1-S3 display the true values and neural network estimations of network efficiency at the different stages of the attacks.

| | **Specific training set** | | | **Training set generalized for Topology and Attack** | | | **Training set generalized for topology, attack, and $\bar{k}$** | | |
|---|---|---|---|---|---|---|---|---|---|
| | **Active** | **Idle** | **Active & Idle** | **Active** | **Idle** | **Active & Idle** | **Active** | **Idle** | **Active & Idle** |
| **Scale-Free / Degree / $\bar{k} = 3$** | 0.02 ± 0.03 | 0.10 ± 0.10 | 0.01 ± 0.01 | 2.39 ± 0.99 | 1.09 ± 0.56 | 0.13 ± 0.04 | 7.36 ± 1.70 | 1.07 ± 0.59 | 0.08 ± 0.04 |
| **Scale-Free / Spreading / $\bar{k} = 12$** | 0.08 ± 0.04 | 0.13 ± 0.08 | 0.05 ± 0.03 | 1.30 ± 0.53 | 0.18 ± 0.13 | 0.06 ± 0.04 | 3.79 ± 1.47 | 0.97 ± 0.59 | 0.23 ± 0.09 |
| **Small-World / Spreading / $\bar{k} = 6$** | 0.06 ± 0.04 | 0.14 ± 0.11 | 0.02 ± 0.01 | 0.40 ± 0.21 | 0.66 ± 0.35 | 0.03 ± 0.02 | 1.26 ± 0.53 | 0.89 ± 0.34 | 0.13 ± 0.05 |
| **Small-World / Random / $\bar{k} = 24$** | 0.09 ± 0.09 | 0.15 ± 0.12 | 0.03 ± 0.05 | 0.15 ± 0.12 | 0.21 ± 0.18 | 0.05 ± 0.08 | 0.78 ± 0.16 | 3.20 ± 0.46 | 0.07 ± 0.05 |
| **Random / Degree / $\bar{k} = 3$** | 0.01 ± 0.02 | 0.05 ± 0.07 | 0.006 ± 0.005 | 0.59 ± 0.21 | 0.50 ± 0.26 | 0.14 ± 0.04 | 5.70 ± 1.30 | 5.24 ± 2.21 | 0.09 ± 0.02 |
| **Random / Random / $\bar{k} = 24$** | 0.06 ± 0.07 | 0.15 ± 0.14 | 0.03 ± 0.02 | 0.12 ± 0.09 | 0.22 ± 0.19 | 0.06 ± 0.04 | 0.95 ± 0.34 | 3.24 ± 0.62 | 0.08 ± 0.05 |

**Table S4 -** Sum of squared residuals (SSR) for six combinations of topology, attack, and link density computed using Neural networks with a training set consisting of: (i) a data set including only the topology, attack, and link density data of the same type of the testing set; (ii) a data set including all the three attacks (degree, spreading and random), topologies (Scale-free, Small-World, and Random) for a given link density, and; (iii) a data set including all the three attacks (degree, spreading and random), topologies (Scale-free, Small-World, and Random), and link densities ($\bar{k} = 3, 6, 12, 24$).

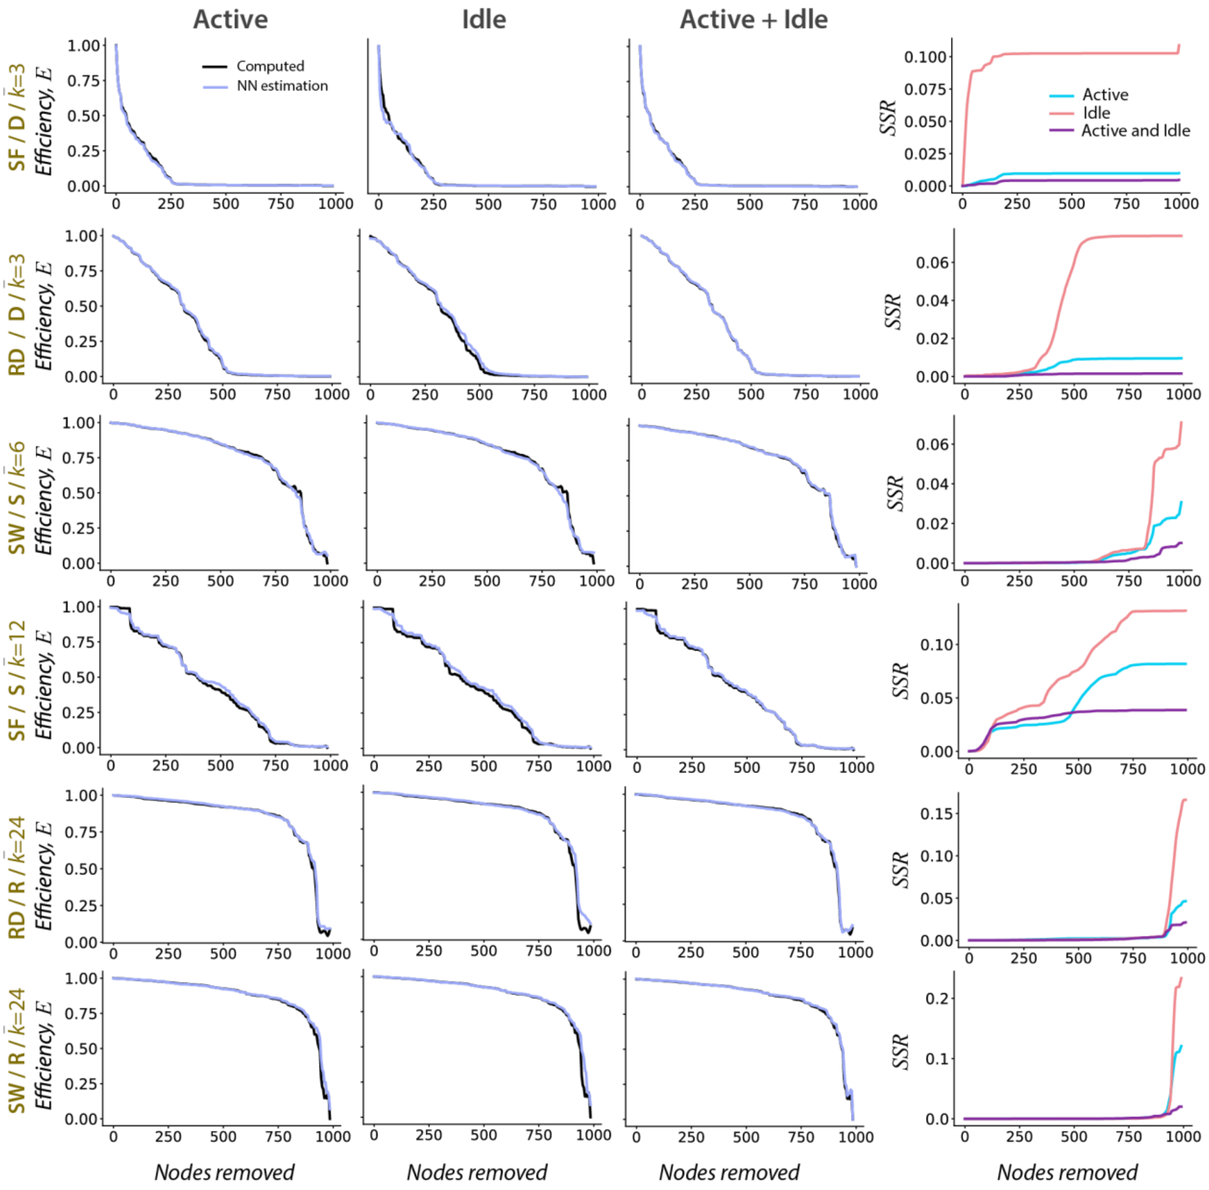


**Fig. S1** - True values (computed) of network efficiency, *E*, and efficiency estimations (NN estimation) obtained from neural networks for different topologies, attacks, and link density combinations. The neural networks were trained with the specific attack (Degree - D, Spreading - S, or Random - R), topology (Scale-free - SF, Small-World - SW, or Random - RD), and link density corresponding to those of the training set. In the rightmost column, the panels display the value of the cumulative SSR as a function of the attack stage for each of the cases.

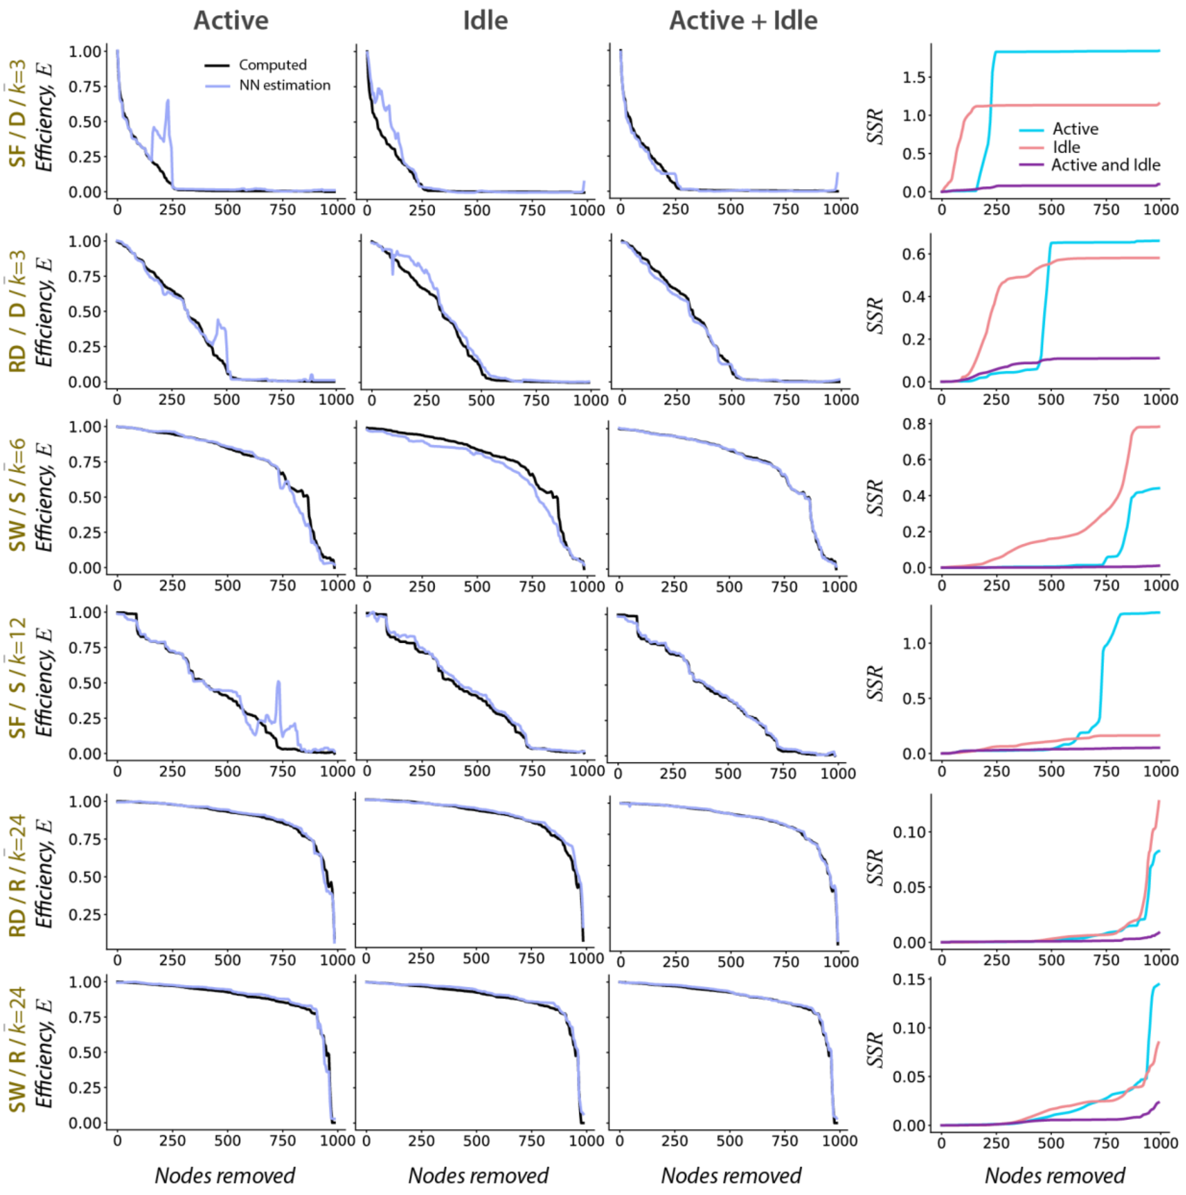


**Fig. S2 -** True values (computed) of network efficiency, $E$, and efficiency estimations (NN estimation) obtained from neural networks for different topologies, attacks, and link density combinations. The neural networks were trained with the augmented dataset consisting of all attacks (Degree - D, Spreading - S, and Random - R) and all topologies (Scale-free - SF, Small-World - SW, and Random - RD) for a given link density. In the rightmost column, the panels display the value of the cumulative SSR as a function of the attack stage for each of the cases.

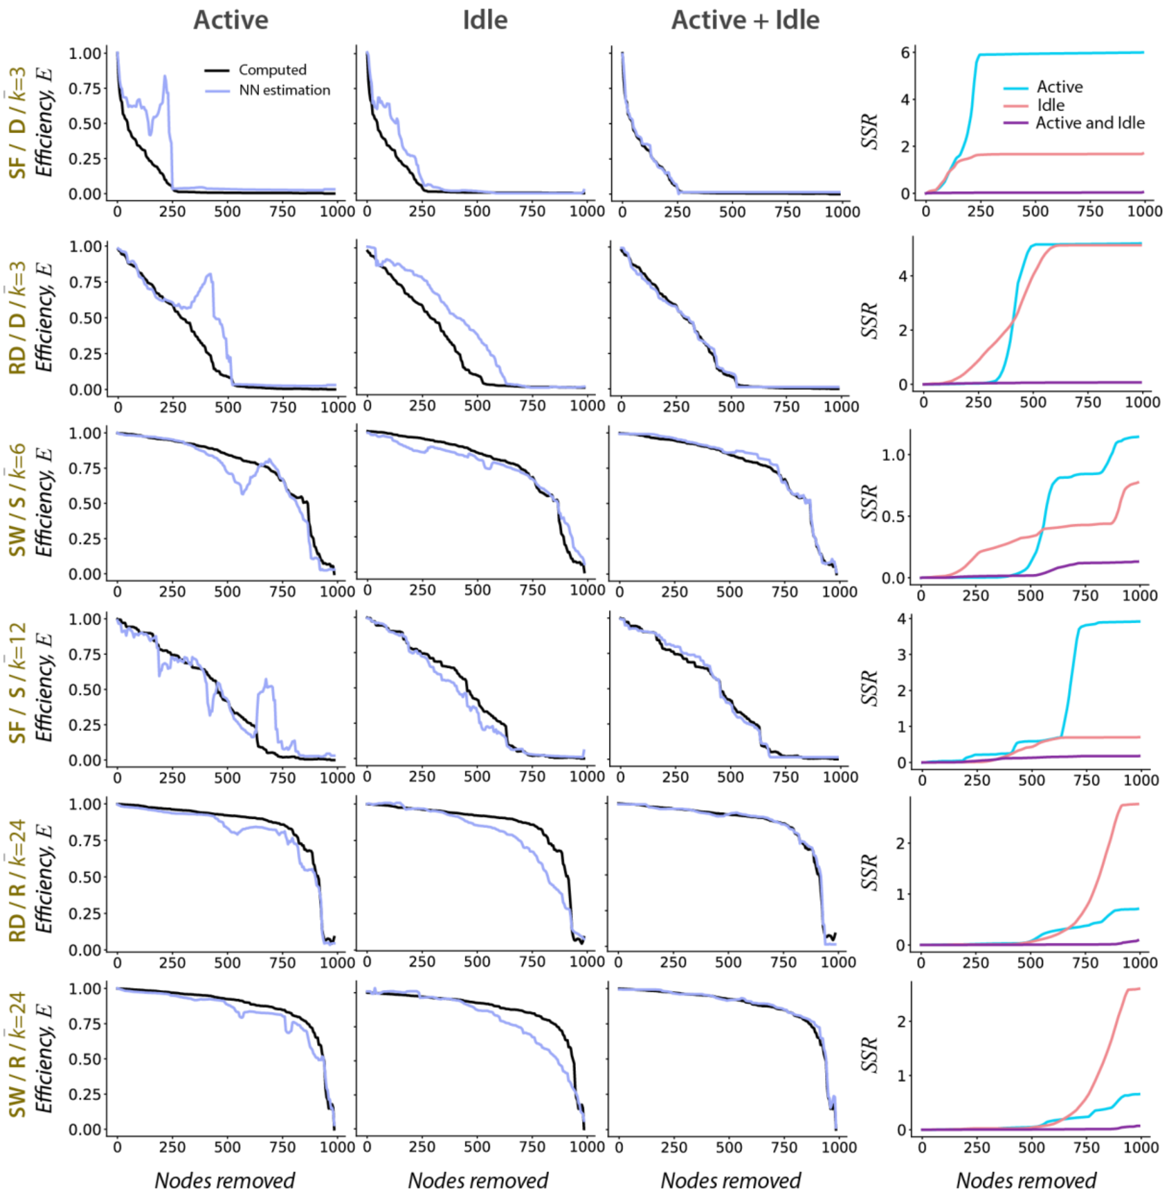


**Fig. S3 -** True values (computed) of network efficiency, $E$, and efficiency estimations (NN estimation) obtained from neural networks for different topologies, attacks, and link density combinations. The neural networks were trained with the augmented dataset consisting of all attacks (Degree - D, Spreading - S, and Random - R), all topologies (Scale-free - SF, Small-World - SW, and Random - RD), and all link density ($\bar{k} = 3, 6, 12, 24$). In the rightmost column, the panels display the value of the cumulative SSR as a function of the attack stage for each of the cases.

## Section E: Neural Network for Real Complex Networks.

This section includes the extended results of the analysis for three other real-world network topologies, namely, the Budapest Connectome [29], Network of flights among the 500 busiest commercial airports in the United States in 2002 [30], and a power grid [1], to test the validity of our hypothesis in more realistic topologies. The results presented in this section were also utilized to evaluate the relevance of Idle information for the model to assess the robustness of the three topologies when they undergo an attack that has not been included in the training set used to fit our model.

Fig. S4 displays the true values and neural network estimations of network efficiencies at the different stages of the attacks. Particularly, for each network topology, the top panels offer the information about the performance of the Neural Networks trained with the different set of indicators (Active, Idle, and Active and Idle) when tested with data corresponding to the same attack type as that used to create the training set (stochastic degree attack). The results clearly support the central hypothesis of this work demonstrating that by also providing Idle information to the model, the accuracy of the estimation of efficiency increases in all the cases and for the most significant part of the attack sequence. The bottom panels for each of the network topologies display the results of the Neural Networks trained using stochastic degree attacks but estimating the decline in efficiency as a different attack type (stochastic betweenness attack) proceeds with the node removal. For both the US airport network and the Budapest Connectome, the inclusion of Idle information in the model increases its estimation power even when evaluated for a previously unseen attack. The performance obtained by the model trained with both Active and Idle indicators for the US airport is particularly remarkable when compared with the resulting performance using either of the two types of indicators alone. However, for the power grid topology, the robustness assessment for a stochastic betweenness attack (previously unseen attack) is worse when estimated with both Active and Idle indicators than that with the Active indicators only. Interestingly, Idle indicators alone yield the most accurate robustness assessment, especially if only the most relevant part of the attack is considered. To understand these apparent discrepancies of the results obtained for the power grid network with respect to all the other network topologies used, we need to better contextualize the particularities of the power grid, which is a network significantly different from the other real and synthetic networks used in this work. Particularly, the power grid network is a low density and spatial network, with no clearly distinguishable hubs. As a stochastic degree attack proceeds in this topology, the Active largest cluster size and link fraction decline very quickly. However, the Idle indicators display an almost negligible trend as the nodes removed at early stages of the attack are dispersed throughout the network (i.e., disconnected nodes in the Idle network). This mismatch in the intrinsic variability of the Active and Idle indicators in the most relevant part of the attack process hinders the neural network in extracting the important information of the Idle indicators, as the range of the Active indicators is overwhelming. In other words, the chosen Idle indictors for low density spatial networks are not suitably encoding complementary information useful for the neural network to increase the accuracy in the estimation. Nevertheless, we want to highlight that the information content in the Idle network is not disputed by these results – recall that the accuracy of the neural network that only uses the Idle indicators is the highest. In this case, the neural network is forced to put weights and bias on the Idle indicators, and this results in an exceedingly good prediction for both the seen attack, and the un-seen attack.

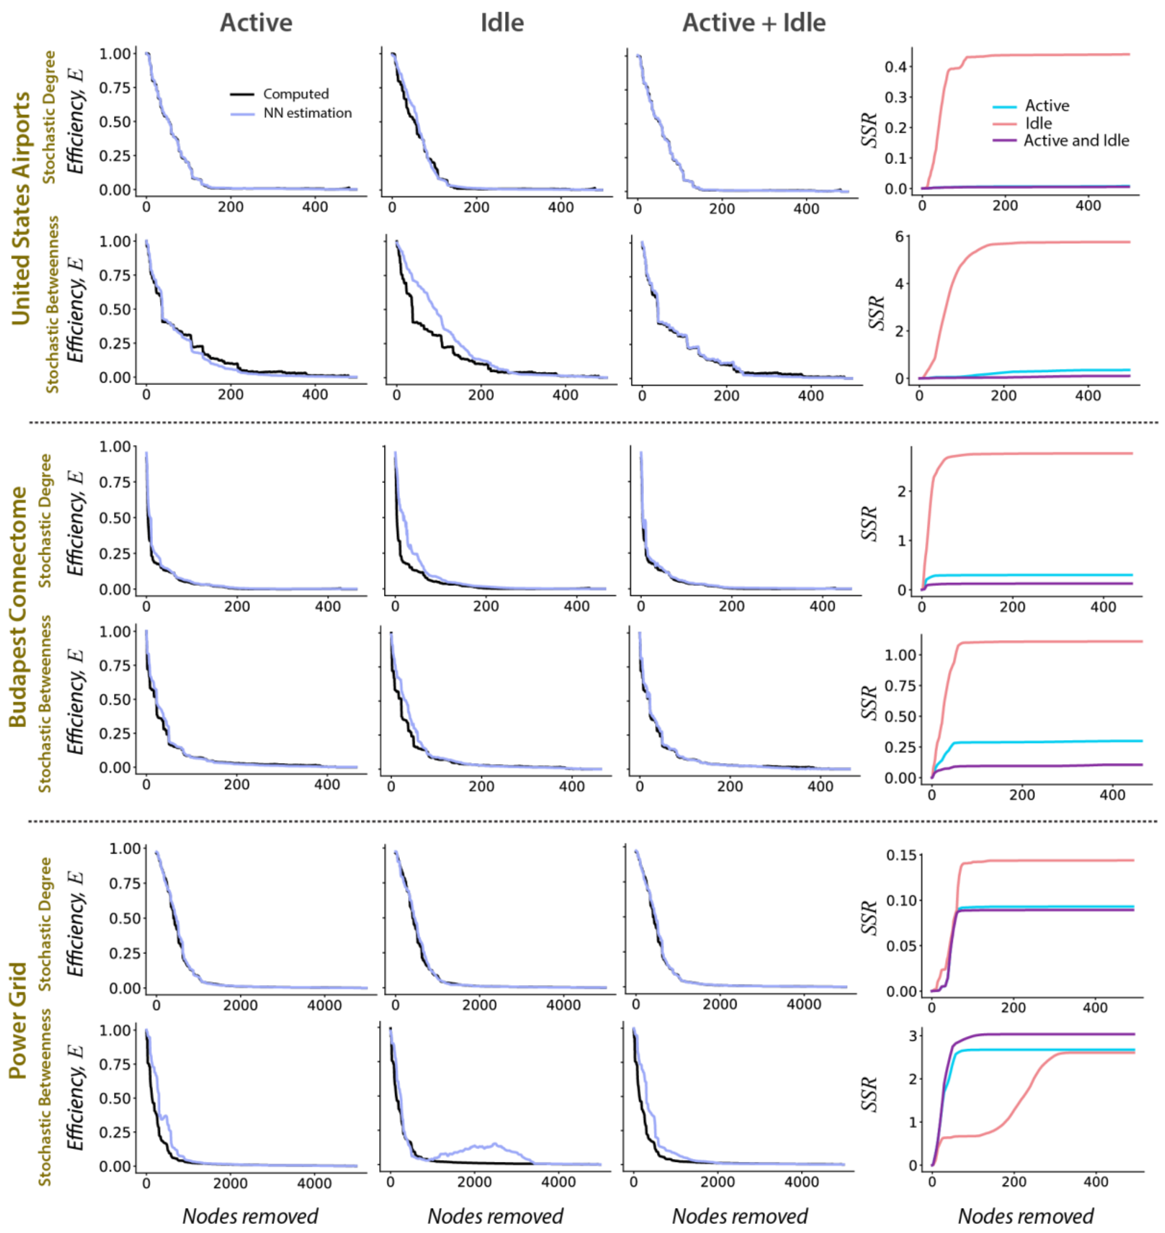


**Fig. S4** - True values (computed) of network efficiency, E, and estimations (NN estimation) of efficiency obtained from neural networks for three real network topologies (US airports, Budapest connectome, power grid). The neural networks were only trained using stochastic targeted attacks for each topology. Still, they were tested for both estimating efficiency as a function of the attack stage when this attack was stochastic targeted attacks and for an unseen attack type, namely, stochastic betweenness attack. In the rightmost column, the panels display the value of the cumulative SSR as a function of the attack stage for each of the cases.
